# Supplementary material for: Topological defect engineering and PT-symmetry in non-Hermitian electrical circuits
Source: arXiv:2011.14836 source file (2020-11-10)
Supplement: Supplementary file 1 [file Supplement.pdf]

## Appendix A: Admittance formalism for periodic circuit arrays

Among the plethora of electric circuit elements which have been developed in the past decades, there are three distinct classes of *linear* elements: resistors, capacitors and inductors. They differ in how a voltage drop $V$ across the element is related to the current $I$ flowing through it. According to Ohm's law, the voltage drop across a resistor is determined by the product of inverse resistance and voltage, $I = \frac{1}{R}V$. For a capacitor, the current relates to the change of voltage across it, $I = C\dot{V}$, where $C$ is the capacitance of the element. The change of the current across an inductor is given by the inverse inductance times the voltage, $\dot{I} = \frac{1}{L}V$.

In the following, we present a formalism [1] to treat periodic structures of linear circuit elements in analogy to known concepts from solid state physics with one important generalization: instead of following the common notion to define the band structure as the mapping from momentum space to energy or frequency eigenvalues, we generalize this approach by considering a mapping from reciprocal space to an arbitrary scalar quantity. In the realm of electric circuits, we use the complex valued admittance, which is the inverse of impedance, to demonstrate this concept. In periodic circuit arrays, a description in terms of the admittance band structure naturally presents itself as it is an easily accessible observable for experimental investigation [1–5].

### 1. Grounded Circuit Laplacian

Consider an electric circuit network with $N$ wire junctions, which we call *nodes* and label by indices from 1 through $N$. Furthermore, ground is referenced by index 0. Each node can be connected to other nodes and/or ground through linear circuit elements. We measure the electric potential (voltage) denoted by $V_j$ with respect to ground at each node. The circuit can be driven through external currents $I_j$ fed into the nodes. We investigate the circuit's response to an AC driving current.

In the frequency domain, currents $I_{jk}(\omega)$ and voltages $V_{jk}(\omega) = V_j(\omega) - V_k(\omega)$ across a linear circuit element are related by complex impedances $Z_{jk}(\omega)$ according to

$$I_{jk}(\omega) = \frac{V_j(\omega) - V_k(\omega)}{Z_{jk}(\omega)}. \tag{A1}$$

For a current $I_{j0}$ leading to ground, voltage $V_0$ is by definition zero, such that $I_{j0}(\omega) = V_j(\omega)/Z_{j0}(\omega)$ remains.

Using Kirchhoff's nodal rule, all currents entering and leaving a node add to zero. This means that the external current $I_j$ fed into each node equals the sum of currents leaving it to other nodes or ground

$$I_j = \sum_{k=0}^{N} I_{jk}. \tag{A2}$$

Inserting (A1) into (A2) now gives a set of relations between the external input currents $I_j(\omega)$ and nodal voltages $V_j(\omega)$ that can be rearranged into the matrix equation

$$J(\omega)\,\boldsymbol{V}(\omega) = \boldsymbol{I}(\omega). \tag{A3}$$

We call $J(\omega)$ the circuit Laplacian [1], it is an $(N \times N)$ matrix with the physical dimension of admittance, the inverse of impedance.

### 2. Admittance band structure

Consider a $d$-dimensional translationally invariant circuit network, i.e. a periodic circuit structure with repeated unit cells reminiscent of the lattice structure of a solid. We label the voltage nodes in such a network by an index tupel $(\boldsymbol{x}, \alpha)$, where the coordinate vector $\boldsymbol{x}$ denotes the position of the unit cell in the lattice and the index $\alpha \in \{1, \ldots, M\}$ represents its sublattice structure.

For a circuit with periodic boundary conditions (PBC), discrete translational invariance leads to a Laplacian which only depends on relative distances,

$$J_{(\boldsymbol{x},\alpha),(\boldsymbol{y},\beta)} = J_{\alpha\beta}(\boldsymbol{x} - \boldsymbol{y}). \tag{A4}$$

Based on this, the unit cell structure of the Laplacian matrix is diagonalized by a spatial Fourier transformation from real to reciprocal space,

$$J_{\alpha\beta}(\boldsymbol{k}) = \sum_{\boldsymbol{x}} J_{\alpha\beta}(\boldsymbol{x})\, \mathrm{e}^{i\,\boldsymbol{k}\cdot\boldsymbol{x}}, \tag{A5}$$

where the right-hand-side sums over all unit cell positions $\boldsymbol{x}$. Upon application of this spatial Fourier transformation, we decompose equation (A3) into Bloch waves characterized by the wave vector $\boldsymbol{k}$. It transforms to a block-diagonal form in $\boldsymbol{k}$-space,

$$J(\boldsymbol{k})\,\boldsymbol{V}(\boldsymbol{k}) = \boldsymbol{I}(\boldsymbol{k}), \tag{A6}$$

where the $(M \times M)$ blocks $J(\boldsymbol{k})$ designate irreducible representations of the discrete translation group. The matrix equation accounts for the remaining sublattice degrees of freedom.

The $M$ eigenvalues of the circuit Laplacian $J(\boldsymbol{k})$ in reciprocal space constitute the admittance band structure $j_m(\boldsymbol{k})$, with $m \in \{1, \ldots, M\}$. The band structure implicitly inherits a parametric dependency on $\omega$ from the circuit Laplacian. We identify the admittance band structure as a mapping $j_m(\boldsymbol{k}) : \mathbb{R}^d \to \mathbb{C}$ from the base manifold of reciprocal wave vectors to the target manifold of admittance eigenvalues of the Laplacian, which are complex-valued scalars. It can be understood as the one-dimensional irreducible representations of the space group of a translationally invariant Laplacian $J$.

a)

b)

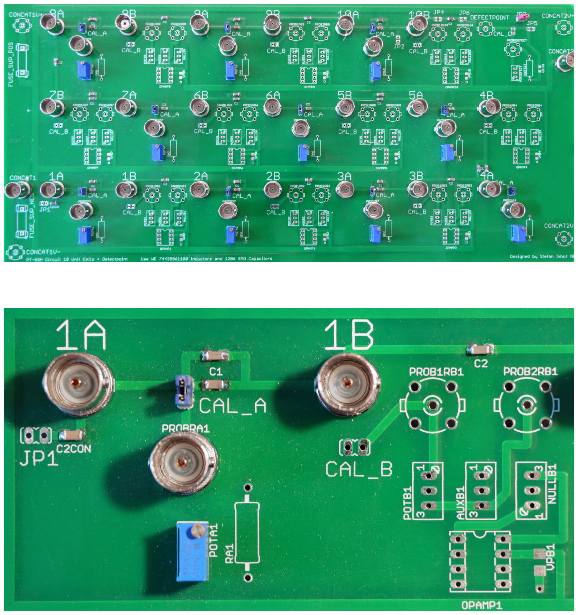


FIG. S1. Circuit board realization of the PT-SSH model. a) Single circuit board containing 10 unit cells. Multiple boards can be connected to create a longer chain. b) Unit cell of the board. Capacitors $C_1$ and $C_2$ realize the hoppings. Inductors on the back of the board connect each node to ground (not shown). The potentiometer realizes the on-site loss term, in the lower right a negative impedance converter can be installed to implement on-site gain, see Appendix G. Note that the labeling on the board is shifted by one site compared to the unit cells used in the main text.

## Appendix B: Experimental setup

The $\mathcal{PT}$-symmetric SSH model is implemented in an electric circuit on the basis of the grounded circuit Laplacian $J(k)$ [1, 2]. Figure S1 shows the circuit board we designed and used in our measurements. We use capacitors $C_1 = 100\,\mathrm{nF}$ and $C_2 = 200\,\mathrm{nF}$ that connect neighboring nodes to implement the two hoppings. The capacitors contribute to the Laplacian as

$$\mathrm{i}\omega \begin{pmatrix} C_1 + C_2 & -C_1 - C_2\,\mathrm{e}^{-\mathrm{i}k} \\ -C_1 - C_2\,\mathrm{e}^{\mathrm{i}k} & C_1 + C_2 \end{pmatrix}. \tag{B1}$$

Each node is connected to ground by an inductor $L = 10\,\mu\mathrm{H}$. This contributes $1/(\mathrm{i}\omega L)\,\mathbb{1}$ to $J(k)$. From the capacitive and inductive terms, the Laplacian has a total diagonal contribution of $\mathrm{i}\omega(C_1 + C_2) + 1/(\mathrm{i}\omega L)$ on each site. From this, we define the circuit's mid-gap frequency $\omega_0 = [(C_1 + C_2)\,L]^{-1/2}$, where the diagonal term cancels. Measured at this frequency, the admittance band structure is centered around zero. The non-Hermitian gain/loss term is realized by resistive elements $R_A$, $R_B$ that connect the first or second node of each unit cell to ground. They contribute to $J(k)$ as $1/2\,\left(R_A^{-1} - R_B^{-1}\right)\sigma_z + 1/2\,\left(R_A^{-1} + R_B^{-1}\right)\mathbb{1} = \left(\mathrm{i}\gamma\,\sigma_z + \mathrm{i}\epsilon\,\mathbb{1}\right)/(\mathrm{i}\omega_0 C_0)$. To prevent the occurrence of dynamical instability outside of the $\mathcal{PT}$-symmetric regime, a constant on-site shift of $\epsilon$ has been applied to the system. In the setup presented in the main text, we chose $\epsilon = -\gamma$, so that $R_A^{-1} = 0$ and $R_B^{-1} = 2\omega_0 C_0 \gamma$. To implement gain (negative resistance), negative impedance converters can be used, which is described in Appendix G.

For our experimental setup, we devised printed circuit boards whose components were pre-selected to show deviations less than 1 % from their nominal values. Our chosen circuit elements are Surface Mount Multilayer Ceramic Chip Capacitors (C1206C104F3GACTU) with C0G dielectric to provide time, voltage and frequency stable capacitance characteristics and WE-HCI SMT High Current Inductors (74435561100, presorted), chosen for minimal inductive coupling between them and low serial resistances ($R_L < 0.5\,\Omega$ for $f < 100\,\mathrm{kHz}$). For the resistive elements, multiturn trimmer resistors (3296W-1-500LF) $R = 50\,\Omega$ are used to be able to modify the resistance.

To investigate the admittance band structure in the different $\mathcal{PT}$ phases, 20 unit cells are connected in a periodic configuration. The AC voltages are measured using lock-in amplifiers (SR530, DSP7625, ITHACO 3961). Based on their specifications, our upper estimate for measurement accuracy is 2%. We use this value to estimate the uncertainty in our computation of the Berry phases in the main text.

For the measurement in the $\mathcal{PT}$ broken regime the trimmer resistors are replaced by fixed resistors with 0.1% tolerance to further decrease disorder efects in the circuit. This is done to observe the transition of the eigenvalues from the imaginary to the real axis more clearly, where no localized defect mode is present.

## Appendix C: $\mathcal{APT}$-symmetry in photonic waveguides

Weimann et al. [6] investigated the $\mathcal{PT}$ symmetric and $\mathcal{PT}$ broken, but not the $\mathcal{APT}$ symmetric phase of the $\mathcal{PT}$ SSH model. Thus they could not observe the re-emergence of the defect state in this regime. In the following we argue why it is challenging to access the $\mathcal{APT}$ phase experimentally in photonic waveguides. For this, we provide an estimate of the shortest coupling length that determines the dynamics for the $\mathcal{APT}$ phase as well as an estimate for the amplitude of the defect state compared to the bulk modes.

### 1. Estimate for the dynamics of the system

The photonic $\mathcal{PT}$-SSH model consists of waveguides written in a glass probe using a femtosecond laser. The different coupling constants are realized by different distances between neighboring waveguides.

Because gain was not available in their implementation, Weimann et. al. [6] were restricted to the on-site potentials 0 and $2\mathrm{i}\gamma$ instead of $\pm\mathrm{i}\gamma$. The maximal loss

that can be implemented using sinusoidal waveguides is about $2\gamma = 1\,\mathrm{cm}^{-1}$. In the $\mathcal{PT}$-SSH model, the conditon to reach the $\mathcal{APT}$-symmetric regime is $\frac{\gamma}{t_1+t_2} > 1$. We further assume $t_1 > t_2$. For an estimate of the shortest coupling length we assume the maximal value for the smaller coupling i.e. $t_2 = 0.25\,\mathrm{cm}^{-1}$. The coupling length $L = \pi/(2t_2)$ is defined as the distance where light is transferred entirely from one waveguide to the other. With our estimate we obtain $\approx 6.3\,\mathrm{cm}$. Therefore, a glass probe of typical length of 15 cm does not provide enough space for sufficiently many waveguides to evolve the necessary dynamics.

### 2. Estimate for the observability of the topological defect state

A second estimate considers the observability of the topological defect state in a photonic waveguide system even if the $\mathcal{APT}$-symmetric regime could be realized. We take a system with the parameters $\gamma = 1\,\mathrm{cm}^{-1}$, $t_1 = 0.249\,\mathrm{cm}^{-1}$ and $t_2 = 0.24\,\mathrm{cm}^{-1}$. The system is then in the $\mathcal{APT}$ symmetric regime. When laser light is sent into the defect site (at $j = (N+1)/2$ for a system consisting of $N$ sites), it will excite not only the defect state mode but also bulk modes. As the defect state is pinned to $\epsilon = -\gamma$, bulk states with smaller damping will overshadow the defect state. To estimate when this happens and how much larger the amplitude of the bulk state will be at the end of the 15 cm probe, we compute the overlap of the initial state $|\Psi_{\mathrm{init}}\rangle = (0, ..., 0, 1, 0, ..., 0)^{\mathrm{T}}$ with the eigenvectors of the Hamiltonian. The overlap with the defect eigenstate is

$$\langle \Psi^{\epsilon}_{\mathrm{defect}} | \Psi_{\mathrm{init}} \rangle = 0.4744, \tag{C1}$$

and the maximal overlap of initial state with the remaining eigenstates is

$$\langle \Psi^{\epsilon}_{i} | \Psi_{\mathrm{init}} \rangle = 0.2796 \quad . \tag{C2}$$

The state with the maximal overlap has an imaginary part of $\mathrm{Im}\,\epsilon_i = -0.8717\,\mathrm{cm}^{-1}$. It is therefore less damped than the defect state. At the end of the probe the amplitude of this state will be about four times larger than the defect state. Hence the intensity will be about 16 times larger than that of the defect state. Therefore the defect state will be much harder to distinguish from the background noise and hence much harder to detect.

This problem cannot be remedied by the use of gain, since this would only contribute a constant factor to all output amplitudes. The relative intensities of the different states, however, are unaffected.

In circuits we measure a steady state response, so that the signal intensity of each eigenstate is proportional only to its associated impedance eigenvalue and not affected by dynamical damping.

## Appendix D: Symmetries of the $\mathcal{PT}$-SSH model

### 1. $\mathcal{PT}$ and $\mathcal{APT}$ symmetry

We investigate two symmetries of the $\mathcal{PT}$-SSH model, $\mathcal{PT}$ and $\mathcal{APT}$. For simplicity, we will use the model Hamiltonian

$$H = \begin{pmatrix} \ddots & t_1 & & & & & \\ t_1 & -\mathrm{i}\gamma & t_2 & & & & \\ & t_2 & \mathrm{i}\gamma & t_1 & & & \\ & & t_1 & -\mathrm{i}\gamma & t_2 & & \\ & & & t_2 & \mathrm{i}\gamma & t_1 & \\ & & & & t_1 & -\mathrm{i}\gamma & t_2 \\ & & & & & t_2 & \ddots \end{pmatrix}, \tag{D1}$$

but all following results hold equally for the rescaled circuit Laplacian $J/i\omega C$. The Hamiltonian's Bloch form is

$$h(k) = (-t_1 - t_2 \cos k)\sigma_x - t_2 \sin k\,\sigma_y + \mathrm{i}\gamma(\omega)\sigma_z, \tag{D2}$$

with $\sigma_i$ the $2 \times 2$ Pauli matrices.

The $\mathcal{PT}$ symmetry is an antiunitary symmetry that commutes with $H$. It is composed of parity transformation $\mathcal{P}:\ x \to -x$ and time reversal $\mathcal{T}$, that acts as complex conjugation $\mathcal{K}$. Its representation in nodal space is

$$\mathcal{PT} = \begin{pmatrix} & & & & & \cdot^{\cdot^{\cdot}} \\ & & & & 1 & \\ & & & 1 & & \\ & & 1 & & & \\ & 1 & & & & \\ 1 & & & & & \\ \cdot^{\cdot^{\cdot}} & & & & & \end{pmatrix} \mathcal{K}. \tag{D3}$$

In Bloch space, the action of the parity transformation $\mathcal{P}$ is $\sigma_x$ on the sublattice and $k \to -k$ on the Brillouin zone. The action of time reversal $\mathcal{T}$ is complex conjugation $\mathcal{K}$ and $k \to -k$. The inversion of reciprocal space from $\mathcal{P}$ and $\mathcal{T}$ cancel out, so the Bloch representation of the $\mathcal{PT}$ transformation is

$$\mathcal{PT} = \sigma_x \mathcal{K}. \tag{D4}$$

The anti-$\mathcal{PT}$ symmetry $\mathcal{APT}$ is the combination of the Hermitian SSH model's chiral symmetry $\mathbb{1} \otimes \sigma_z$ with time reversal $\mathcal{T}$. It is an antiunitarity symmetry and anticommutes with the Hamiltonian of the $\mathcal{PT}$ SSH model. Its representation in nodal space is

$$\mathcal{APT} = \begin{pmatrix} \ddots & & & & & & \\ & 1 & & & & & \\ & & -1 & & & & \\ & & & 1 & & & \\ & & & & -1 & & \\ & & & & & 1 & \\ & & & & & & \ddots \end{pmatrix} \mathcal{K}, \tag{D5}$$

its Bloch representation is

$$\mathcal{APT} = \sigma_z \mathcal{T} = \sigma_z \mathcal{K},\ k \to -k. \tag{D6}$$

### 2. Symmetries of the spectrum and eigenstates

Let us now investigate the implications of these symmetries on the eigenvalues $E(k)$ and eigenstates $\Psi(k)$ of $h(k)$. From the eigenvalue equation $h(k)\,\Psi(k) = E(k)\,\Psi(k)$ and $[\mathcal{PT}, h(k)] = 0$, we obtain

$$\begin{aligned} E(k)\,\Psi(k) = h(k)\,\Psi(k) = \\ = h(k)\,(\mathcal{PT})^2\,\Psi(k) = \mathcal{PT}\,h(k)\,(\mathcal{PT}\,\Psi(k)). \end{aligned} \tag{D7}$$

Multiplying $\mathcal{PT}$ from the left then gives

$$\begin{aligned} \mathcal{PT}\,E(k)\,\Psi(k) = (E(k))^*\,(\mathcal{PT}\,\Psi(k)) = \\ = h(k)\,(\mathcal{PT}\,\Psi(k)) = \bar{E}(k)\,\bar{\Psi}(k). \end{aligned} \tag{D8}$$

This means that for every eigenstate $\Psi(k)$, there is another eigenstate $\bar{\Psi}(k) = \mathcal{PT}\,\Psi(k)$ with eigenvalue $\bar{E}(k) = E^*(k)$. There now exist two possibilities. The first case is that $\Psi(k)$ is symmetric under $\mathcal{PT}$, so that $\Psi(k)$ and $\bar{\Psi}(k)$ are the same state. This is the case if $E(k)$ is real-valued. The second case arises when $E(k)$ is complex-valued. Then $E$ and $\bar{E} = E^*$ differ, so that $\Psi(k)$ and $\bar{\Psi}(k)$ are distinct and transform into another under $\mathcal{PT}$. This behavior arises because $\mathcal{PT}$ is an antiunitary operator, so it does not generally commute with scalars such as $E(k)$. These two different realizations of $\mathcal{PT}$ symmetry in the eigenstates are why symmetry phase transitions exist in the $\mathcal{PT}$ SSH model.

Repeating the above calculation for $\mathcal{APT}$ symmetry, using $\{\mathcal{APT}, h(k)\} = 0$, gives another relation between pairs of eigenvalues, $\bar{E} = -E^*$. Here, the corresponding eigenstates are symmetric under $\mathcal{APT}$ if their eigenvalues are purely imaginary.

Together, these two symmetries constrain the spectrum to be symmetric under reflection around both the real and imaginary axis in the complex plane. For a two-band model, this condition can only be fulfilled if the two eigenvalues are purely real or imaginary, so the resulting eigenstates are always either $\mathcal{PT}$ or $\mathcal{APT}$ symmetric. This is reflected in the expression of the band structure (3), that is a square root of a real-valued argument, so it can only produce purely real or imaginary eigenvalues.

### 3. Symmetries and the defect state

When the defect site is introduced to the center of the $\mathcal{PT}$-SSH chain, its total number of sites becomes odd. From the symmetry constraints, it follows that this state must be at zero eigenvalue, since only an even number of them can form pairs under reflection about the real or imaginary axis. Accordingly, this state must be both $\mathcal{PT}$ and $\mathcal{APT}$ symmetric. If the band structure is gapped at zero, the state is necessarily localized. Since $\mathcal{PT}$ inverts real space, this state must then be centered around the central defect site.

## Appendix E: $\mathcal{PT}$ winding number

A topological classification of $\mathcal{PT}$ symmetric models can be derived directly from the $\mathcal{PT}$ operator, that generalizes the Zak phase classification to $\mathcal{PT}$ breaking regimes. For this, we define the $\mathcal{PT}$ winding number

$$\mathcal{W}_n^{\mathcal{PT}} = \frac{1}{2\pi} \oint_{\mathrm{BZ}} \mathrm{d}k\, \partial_k \arg\left\{\Psi_n^\dagger(k)\,\mathcal{PT}\,\Psi_n(k)\right\}. \tag{E1}$$

Due to the antiunitarity of $\mathcal{PT}$, a gauge transformation $\Psi_n(k) \to \mathrm{e}^{\mathrm{i}\theta_n(k)}\Psi_n(k)$ can only result in a factor of $\mathrm{e}^{-2\mathrm{i}\theta_n(k)}$ in the scalar product of (E1). This means that it can only change the winding number by multiples of two, so that the $\mathcal{PT}$ winding number induces a $\mathbb{Z}_2$ classification for bands.

### 1. $\mathcal{PT}$ symmetric phase

In the following, we show that for a $\mathcal{PT}$ symmetric band with states $\Psi(k)$, this winding number is equivalent to the Zak phase. Since $\mathcal{PT}$ is antiunitary and squares to $\mathbb{1}$, it acts on a $\mathcal{PT}$ symmetric state as a phase factor $\mathcal{PT}\Psi = \mathrm{e}^{\mathrm{i}\varphi}\Psi$. Since both $\mathcal{P}$ and $\mathcal{T}$ invert reciprocal space, $\mathcal{PT}$ leaves the wave number $k$ invariant. Using these properties, we obtain

$$\begin{aligned} 0 =& \partial_k(\Psi^\dagger(k)\Psi(k)) \\ =& \left(\partial_k\Psi^\dagger(k)\right)\Psi(k) + \Psi^\dagger(k)\partial_k\Psi(k) \\ =& (\mathcal{PT}\Psi(k))^\dagger\partial_k\mathcal{PT}\Psi(k) + \Psi^\dagger(k)\partial_k\Psi(k) \\ =& \mathrm{i}\partial_k\varphi(k) + 2\Psi^\dagger(k)\partial_k\Psi(k) \\ \Longrightarrow& \frac{1}{2}\partial_k\varphi(k) = \mathrm{i}\Psi^\dagger(k)\partial_k\Psi(k). \end{aligned} \tag{E2}$$

This means that the Berry connection of a given $\mathcal{PT}$ symmetric band is equal to half the gradient of the states' phase factor $\varphi(k)$ under $\mathcal{PT}$ transformation. For $\mathcal{PT}$ symmetric states $\mathcal{PT}\,\Psi_n(k) = \mathrm{e}^{i\varphi_n(k)}\Psi_n(k)$, (E1) simplifies to

$$\mathcal{W}_n^{\mathcal{PT}} = \frac{1}{\pi}\oint_{\mathrm{BZ}} \mathrm{d}k\,\frac{1}{2}\,\partial_k\varphi_n(k) \tag{E3}$$

which, using (E2), equals the Zak phase divided by $\pi$. We see that in this regime, the Zak phase's $\pi$ quantization is protected by $\mathcal{PT}$ symmetry.

### 2. Broken $\mathcal{PT}$ symmetry

As discussed in Appendix D, the eigenstates of a $\mathcal{PT}$ symmetric model can spontaneously break $\mathcal{PT}$. Then,

they must occur in pairs $\Psi_+$, $\Psi_-$. In this case, the previously discussed identity between the $\mathcal{PT}$ winding and the Zak phase is no longer valid. This is in line with the measured Berry phases described in the main text, which lose $\pi$ quantization in the $\mathcal{PT}$ broken and $\mathcal{APT}$ symmetric regimes.

In the $\mathcal{PT}$ broken regime, the band structure of the $\mathcal{PT}$-SSH model is split into a section with $\mathcal{PT}$ symmetric eigenstates

$$\Psi_\pm \ \mathcal{PT}\text{-symmetric:} \ \ \mathcal{PT}\,\Psi_\pm = \mathrm{e}^{\mathrm{i}\varphi_\pm}\,\Psi_\pm \tag{E4}$$

and a section with $\mathcal{PT}$-breaking eigenstates

$$\Psi_\pm \ \mathcal{PT}\text{-broken:} \ \ \mathcal{PT}\,\Psi_\pm = \mathrm{e}^{\mathrm{i}\varphi}\,\Psi_\mp. \tag{E5}$$

Note that in the latter case both transformations $\Psi_+ \xrightarrow{\mathcal{PT}} \Psi_-$ and $\Psi_- \xrightarrow{\mathcal{PT}} \Psi_+$ produce the same phase factor $\mathrm{e}^{\mathrm{i}\varphi}$, which follows from the antiunitarity of $\mathcal{PT}$. The two sections of the band structure meet at the exceptional points, where $\Psi_\pm$ coalesce into one vector.

Despite the presence of a gap closing at the exceptional point, the $\mathcal{PT}$ winding is still well-defined. To show this, choose a gauge where the integral $\int \mathrm{d}k\,\partial_k \arg\{\Psi^\dagger_\pm(k)\ \Psi_\mp(k)\}$ over the $\mathcal{PT}$ broken section of the band vanishes, which is always possible since $\Psi_+(k)$ and $\Psi_-(k)$ have independent gauge. From (E5), we see that the contribution of the $\mathcal{PT}$ broken section to the $\mathcal{PT}$ winding number

$$\begin{aligned}
&\int \mathrm{d}k\,\partial_k \arg\{\Psi^\dagger_\pm(k)\mathcal{PT}\Psi_\pm(k))\} \\
&= \int \mathrm{d}k\,\partial_k \arg\{\Psi^\dagger_\pm(k)\mathrm{e}^{\mathrm{i}\varphi(k)}\Psi_\mp(k)\} \\
&= \int \mathrm{d}k\,\partial_k \left(\arg\{\mathrm{e}^{\mathrm{i}\varphi(k)}\} + \arg\{\Psi^\dagger_\pm(k)\Psi_\mp(k)\}\right) \\
&= \int \mathrm{d}k\,\partial_k(k)\,\varphi(k)
\end{aligned} \tag{E6}$$

is equal for both bands, so that it does not matter how one chooses to continue individual bands at the exceptional point. It follows that the $\mathcal{PT}$ winding number is uniquely defined in all symmetry phases of our model.

### 3. Edge states

For $\mathcal{PT}$ symmetric two-band models, the edge state is an eigenstate of $\mathbb{1}\otimes\sigma_z$, so that it only experiences a shift in eigenvalue upon the introduction of a gain/loss term [7]. In the following, we show that the $\mathcal{PT}$ winding is also insensitive to the $\sigma_z$ term, so that both the presence or absence of edge states and the $\mathcal{PT}$ winding number can be traced back to the Zak phase classification of the Hermitian case.

Consider that the $\mathcal{PT}$ winding number can only change if the $\mathcal{PT}$ inner product $\Psi^\dagger(k)\mathcal{PT}\Psi(k)$ crosses zero for some value of $k$. In our two-band model, an eigenstate $\Psi(k)$ can be represented by a vector $(u(k), v(k))^\intercal$. Thus the $\mathcal{PT}$ inner product can be written as

$$\begin{aligned}
\Psi^\dagger\mathcal{PT}\Psi &= (u^*, v^*)\ \sigma_x\,\mathcal{K}\,(u, v)^\intercal \\
&= 2\,u^*\,v^*.
\end{aligned} \tag{E7}$$

This expression can only be zero if either $u$ or $v$ vanish. This can only occur when at least one of the $2\times 2$ Bloch-Hamiltonian's off-diagonal elements is zero, since otherwise $(1,0)^\intercal$ and $(0,1)^\intercal$ cannot be eigenvectors. In a $\mathcal{PT}$ symmetric two-band model, the non-Hermitian term is proportional to $\sigma_z$, so it cannot affect the Hamiltonian's off-diagonal elements and as such can't cause a change of the $\mathcal{PT}$ winding number. This means that both the presence of edge states and the $\mathcal{PT}$ winding number are unaffected by the non-Hermitian term, so a non-trivial $\mathcal{PT}$ winding number predicts the presence of edge states in a $\mathcal{PT}$ symmetric two-band model.

## Appendix F: Complex $k$ in localized states

Consider a periodic hopping model with hoppings only within and between neighbouring unit cells. The spatial evolution of an eigenstate $\Psi$ in such a lattice is given by the eigenvalue problem $H\Psi = \epsilon\Psi$, which can be written as a difference equation

$$H_{-1}\Psi_{n-1} + H_0\Psi_n + H_1\Psi_{n+1} = \epsilon\Psi_n. \tag{F1}$$

$H_{-1}$, $H_0$ and $H_1$ are blocks of the Hamiltonian describing the hopping terms to the left ($H_{-1}$), right ($H_1$) or within the unit cell ($H_0$). $\Psi_n$ is the part of vector $\Psi$ that belongs to the $n$-th unit cell. An exponential ansatz $\Psi_n = \mathrm{e}^{\mathrm{i}kn}\Psi_0$, $k\in\mathbb{C}$ can be used to solve the difference equation. Inserting this and dividing by $\mathrm{e}^{\mathrm{i}kn}$, we obtain

$$\left(H_{-1}\mathrm{e}^{-\mathrm{i}k} + H_0 + H_1\mathrm{e}^{\mathrm{i}k}\right)\Psi_0 = \epsilon\Psi_0 \tag{F2}$$

$$\iff h(k)\,\Psi_0 = \epsilon\Psi_0. \tag{F3}$$

The matrix on the left of (F2) is identical to the Bloch-Hamiltonian $h(k)$ as obtained from Fourier transformation. This derivation justifies that inserting complex values of $k$ into the Bloch Hamiltonian yields exponentially growing or decaying states that solve the eigenvalue problem in the system's bulk region. In a lattice of infinite size or with periodic boundary conditions, only states with real-valued $k$ can satisfy the conditions of normalizability or periodicity, respectively. Accordingly, the eigenstates in this case are given by the band structure of real-valued $k$. However, with open boundary conditions or in the presence of defects, exponentially localized states can arise. These states then correspond to solutions to (F3) with complex valued $k$ since they still need to solve (F1) away from the boundary/defect sites.

## Appendix G: Balanced gain-loss implementation

In an electrical circuit, gain can be implemented by negative impedance converters. This way, the circuit

can be tuned as close to actual $\mathcal{PT}$ symmetry as the precision of its components allows. Balanced gain and loss circuit implementations have been previously realized for other models in [8, 9]. For the sets of measurements we presented in the main text, including gain was not feasible: Whenever edge states or $\mathcal{PT}$ breaking bulk states are present, the circuit would become dynamically unstable. We did, however, perform a set of measurements for periodic boundary conditions in a balanced gain-loss configuration. Figure S2b) shows a diagram of the negative impedance converter used to implement gain. We measured the band structure for effective resistances $R_A = -25\,\Omega$ and $R_B = 20\,\Omega$. Since disorder and imprecision of real circuit elements always breaks $\mathcal{PT}$ to some degree, a small loss envelope is still necessary to stabilize the system, which is why the absolute values of $R_A$ and $R_B$ differ slightly. Figure S2a) shows the measured band structure. No loss-envelope correction has been applied to the depicted eigenvalues. As we can see, the imaginary part is close to zero, with only a slight shift that prevents dynamical instability.

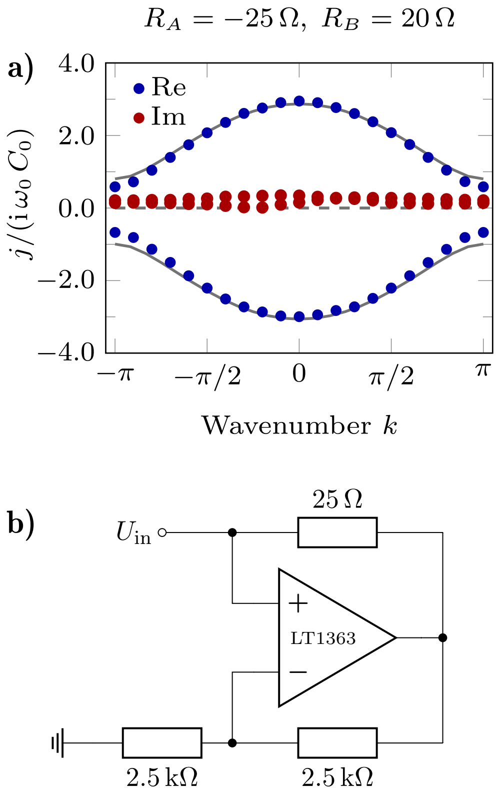


FIG. S2. Implementation of the circuit with balanced gain and loss. a) Theoretic and measured admittance bandstructure of the $\mathcal{PT}$ SSH chain in the $\mathcal{PT}$ symmetric regime, using actual gain through negative impedance converters. Circuit parameters $C_1 = 100\,\mathrm{nF}$, $C_2 = 200\,\mathrm{nF}$, $L = 10\,\mu\mathrm{H}$, $R_A = -25\,\Omega$ and $R_B = 20\,\Omega$ were used. The values are not corrected by a loss envelope. b) Schematic of the negative impedance converter. From input node at voltage $U_{\mathrm{in}}$, the circuit appears as an effective negative resistor of $-25\,\Omega$ to ground.

[1] C. Lee, S. Imhof, C. Berger, F. Bayer, J. Brehm, L. Molenkamp, T. Kiessling, and R. Thomale, Commun. Phys. **1**, 39 (2018).
[2] T. Helbig, T. Hofmann, C. H. Lee, R. Thomale, S. Imhof, L. W. Molenkamp, and T. Kiessling, Phys. Rev. B **99**, 161114 (2019).
[3] T. Helbig, T. Hofmann, S. Imhof, M. Abdelghany, T. Kiessling, L. W. Molenkamp, C. H. Lee, A. Szameit, M. Greiter, and R. Thomale, Nat. Phys. **16**, 747 (2020).
[4] S. Imhof, C. Berger, F. Bayer, J. Brehm, L. W. Molenkamp, T. Kiessling, F. Schindler, C. H. Lee, M. Greiter, T. Neupert, and R. Thomale, Nat. Phys. **14**, 925 (2018).
[5] T. Hofmann, T. Helbig, F. Schindler, N. Salgo, M. Brzezińska, M. Greiter, T. Kiessling, D. Wolf, A. Vollhardt, A. Kabaši, C. H. Lee, A. Bilušić, R. Thomale, and T. Neupert, Phys. Rev. Research **2**, 023265 (2020).
[6] S. Weimann, M. Kremer, Y. Plotnik, Y. Lumer, S. Nolte, K. G. Makris, M. Segev, M. C. Rechtsman, and A. Szameit, Nat. Mater. **16**, 433 (2016).
[7] K. Esaki, M. Sato, K. Hasebe, and M. Kohmoto, Phys. Rev. B **84**, 205128 (2011).
[8] J. Schindler, A. Li, M. C. Zheng, F. M. Ellis, and T. Kottos, Phys. Rev. A **84**, 040101 (2011).
[9] Y. Choi, C. Hahn, J. W. Yoon, and S. H. Song, Nat. Commun. **9**, 2182 (2018).
